# Supplementary material for: Learned Localized Mesh Refinement
Source: arXiv:2609.31946 source file (2026-09-25)
Supplement: Supplementary file 1 [file supp.tex]

%%%% Large single column format, used for IMWUT, JOCCH, PACMPL, POMACS, TAP, PACMHCI
% \documentclass[acmlarge,screen]{acmart}

%%%% Large double column format, used for TOG
% SIGGRAPH:
% \documentclass[acmtog,anonymous,review,nonacm]{acmart}
% \documentclass[acmtog,review,nonacm]{acmart}
\documentclass[acmtog]{acmart}
% \documentclass[acmtog,anonymous,review, draft, nonacm]{acmart} % use "draft" to switch off figure rendering for compilation speed
% \acmSubmissionID{1871}
%\documentclass[sigconf]{acmart}
% arXiv:
% \documentclass[acmtog,nonacm]{acmart}

\input{text/0_preamble}

%%
%% end of the preamble, start of the body of the document source.

\begin{document}

%%
%% The "title" command has an optional parameter,
%% allowing the author to define a "short title" to be used in page headers.
\title{Learned Localized Mesh Refinement}

%%
%% The "author" command and its associated commands are used to define
%% the authors and their affiliations.
%% Of note is the shared affiliation of the first two authors, and the
%% "authornote" and "authornotemark" commands
%% used to denote shared contribution to the research.
\author{Xiao Zhan}
\orcid{0000-0002-1825-0097}
\affiliation{
  \institution{Massachusetts Institute of Technology (MIT)}
  \city{Cambridge}
  \state{Massachusetts}
  \country{USA}
}
\email{zhanx@mit.edu}

\author{Chrystiano Ara\'{u}jo}
\orcid{0000-0002-8237-9426}
\affiliation{
  \institution{Roblox}
  \city{San Mateo}
  \state{California}
  \country{USA}
}
\email{caraujo@roblox.com}

\author{Kangle Deng}
\orcid{0009-0000-0565-4255}
\affiliation{
  \institution{Roblox}
  \city{San Mateo}
  \state{California}
  \country{USA}
}
\email{kdeng@roblox.com}

\author{Maneesh Agrawala}
\orcid{0000-0002-8996-7327}
\affiliation{
  \institution{Stanford}
  \city{Stanford}
  \state{California}
  \country{USA}
}
\email{maneesh@cs.stanford.edu}

\author{Hsueh-Ti Derek Liu}
\orcid{0009-0001-1753-4485}
\affiliation{
  \institution{Roblox}
  \city{Vancouver}
  \state{British Columbia}
  \country{Canada}
}
\email{hsuehtiliu@roblox.com}

\author{Mina Konakovi\'{c} Lukovi\'{c}}
\orcid{0000-0002-2895-0206}
\affiliation{
  \institution{Massachusetts Institute of Technology (MIT)}
  \city{Cambridge}
  \state{Massachusetts}
  \country{USA}
}
\email{minakl@mit.edu}

%% By default, the full list of authors will be used in the page
%% headers. Often, this list is too long, and will overlap
%% other information printed in the page headers. This command allows
%% the author to define a more concise list
%% of authors' names for this purpose.
% \renewcommand{\shortauthors}{Anonymous Author(s)}

\maketitle

\input{text/8_supp}

\clearpage

\bibliographystyle{ACM-Reference-Format}
\bibliography{bibliography}

\end{document}
